# Supplementary material for: Option Transfer and SMDP Abstraction with Successor Features
Source: arXiv:2110.09196 source file (2022-06-08)
Supplement: Supplementary file 1 [file appendix_cumulants.tex]

\section{Relation to Cumulants}

In this section, we discuss the relation between our feature-matching IRL algorithm with the cumulant formulation from Option Keyboard.

The option keyboard relies on extended cumulants defined on the state, action and history, that is, $e_i(s, h, a)$. In particular, the history can be used to account for the features that are accumulated so far and determine whether the option shall stop: $Q(s, h, a_\tau) \geq Q(s, h, a_{\neq \tau}) \implies \beta(s, h, t) = 1$. This encoding has the advantage of taking into account the history (e.g., specifying $k$-steps to stop the option). However, manually crafting the extended cumulants as a function of history then applying Q-learning to find suitable policies can be problematic.

In our case, we utilize inverse RL (in particular the LP formulation) to account for the history through occupancy measures $\mu_{s,a}$, and hence the termination arises naturally from the optimisation objective. Moreover, this may allow us to express more flexible objectives. The LP formulation is as follows:

\begin{align}
    \textnormal{maximise}_{\mu_{s,a}} \quad &f(\mu_{s,a}, \theta_{s,a})\\
    \textnormal{subject to } &\sum_{a}\mu_{s,a} = \gamma\sum_{s', a'} \mu_{s', a'} P(s|s', a') &\forall s\in S\\
    &\mu_{s,a} \geq 0 &\forall s\in S, a\in A
\end{align}

where the aggregation function $f$ specify the objective of the (option) policy. 

For example, the occupancy measure found for $f(\mu_{s,a}, \theta_(s,a)) = \sum_{s,a} \mu_{s,a} w_r^T\bm{\theta}(s,a)$ induces an equivalent policy maximising $V^\pi$ with the reward function $r(s,a) = w_r^T\bm{\theta}(s,a)$.

In our case where we aim for the cumulative feature expectation to match that of an expert, the objective is defined as $f(\mu_{s,a}, \theta_{s,a}) = |\sum_{s,a}\mu_{s,a} \bm{\theta}(s,a) - \bm{\psi}^{\bar{o}}|$. Since the action space is augmented with the terminate action $a_\tau$, the induced policy $\pi^o(a|s) = \frac{\mu_{s,a}}{\sum_{a}{\mu_{s,a}}}$ will include the termination action. This objective introduces an AND relation on all features $\bm{\theta} = \{\theta_0, ... \theta_k\}$ matching the expert.

In general, we (can? or is this not correct?) can define broader class of objective functions. For example, the aforementioned objective $f(\mu_{s,a}, \theta_(s,a)) = \sum_{s,a} \mu_{s,a} w_r^T\bm{\theta}(s,a)$ which aims to maximise the return with preference vector $\bm{w}_r$. This objective function correspond to the preferences specified by combined cumulants, excluding the termination condition of an option.

To express an OR-like condition, we can define a preference vector $\bm{w}_r$ together with a threshold $c$. For example, given features of key, door, star as $\bm{w}_r = (1, 0, 1)$, we define the objective as $f(\mu_{s,a}, \theta_(s,a)) = |\sum_{s,a} \mu_{s,a} \bm{w}_r^T\bm{\theta}(s,a) - c|$ with $c=1$. In this way, the option will either find a key or find a star then terminate itself. 

To include negative preferences, we can augment the objective with the penalty weights: $f(\mu_{s,a}, \theta_(s,a)) = |\sum_{s,a} \mu_{s,a} \bm{w}_r^T\bm{\theta}(s,a) - c| - \sum_{s,a} \mu_{s,a} \bm{w}_\textnormal{penalty}^T\bm{\theta}(s,a) $.

\subsection{Expressing abstract successor options as cumulants}
The feature-matching options can be modelled by cumulants. Given an expert feature $\bm{\psi}^{\bar{o}}$, the cumulants (pseudo-rewards) can be defined as:
\begin{align}
    e_i(s, h, a) = 
    \begin{cases}
    1 &\textnormal{if } |\bm{\psi}_h - \bm{\psi}^{\bar{o}}| \leq \epsilon \textnormal{ and } a = a_\tau\\
    0 &\textnormal{otherwise}
    \end{cases}
\end{align}
where $\bm{\psi}_h = \sum_{(s_t,a_t) \sim h} \gamma^t\bm{\theta}(s_t,a_t)$ is the successor feature achieved by the agent.
